# Supplementary material for: Multimodal Maximum Entropy Dynamic Games
Source: arXiv:2201.12925 source file (2022-02-02)
Supplement: Supplementary file 1 [file supplementary.tex]

\documentclass{article}

\input{paper/math_commands}
\input{paper/packages}

\usepackage[margin=1in]{geometry}
\usepackage{placeins}
\usepackage{tocloft}

\title{Supplementary Material}
\date{}
\begin{document}
\maketitle
\addtolength{\cftsubsecnumwidth}{20pt}
\addtolength{\cftsecnumwidth}{20pt}
\tableofcontents

\include{paper/supplementary_main}

\FloatBarrier
\bibliographystyle{unsrtnat}
\bibliography{references}

\end{document}
